# Supplementary material for: Memory-Optimized Once-For-All Network
Source: arXiv:2409.05900 source file (2024-09-05)
Supplement: Supplementary file 1 [file A_Formalization.tex]

\section{Memory Usage Formalization}
\label{app:memory_formalization}

We formalize the memory usage for a Mobile Inverted Bottleneck (MB) block. Let us define the following parameters:

\begin{itemize}
    \item $E$: expand ratio factor
    \item $K$: kernel size of the convolution
    \item $S$: stride (2 for the last block of a stage, 1 otherwise)
    \item $C_{in}$: number of input channels
    \item $C_{out}$: number of output channels
    \item $I$: input feature map size
\end{itemize}

The memory complexity for each layer in the MB block can be expressed as follows:

\subsection{Expansion Convolution Layer}
\begin{equation}
    M_{exp} = \underbrace{O(C_{in}I^2)}_\text{input memory} + \underbrace{O(C_{in}EC_{in})}_\text{weight memory} + \underbrace{O(EC_{in}I^2)}_\text{output memory}
\end{equation}

Where input memory stores the initial feature map, weight memory holds the learnable parameters, and output memory stores the expanded feature map.

\subsection{Depthwise Convolution Layer}
\begin{equation}
    M_{dw} = \underbrace{O(EC_{in}I^2)}_\text{input memory} + \underbrace{O(EC_{in}K^2)}_\text{weight memory} + \underbrace{O(EC_{in}(\frac{I}{S})^2)}_\text{output memory}
\end{equation}

Here, input memory stores the expanded feature map, weight memory contains the depthwise convolution kernels, and output memory holds the spatially convolved features.

\subsection{Projection Convolution Layer}
\begin{equation}
    M_{proj} = \underbrace{O(EC_{in}(\frac{I}{S})^2)}_\text{input memory} + \underbrace{O(EC_{in}C_{out})}_\text{weight memory} + \underbrace{O(C_{out}(\frac{I}{S})^2)}_\text{output memory}
\end{equation}

In this layer, input memory stores the depthwise convolved features, weight memory holds the projection convolution parameters, and output memory contains the final output feature map.

Note that within a stage (where $S=1$ and $C_{in}=C_{out}$), we observe $M_{exp} = M_{proj}$.
