# Supplementary material for: Memory-Optimized Once-For-All Network
Source: arXiv:2409.05900 source file (2024-09-05)
Supplement: Supplementary file 2 [file B_Equations.tex]

\section{Channel Size Optimization for Memory-Constant Architecture}
\label{app:channel_optimization}

Our objective is to optimize channel sizes across stages to achieve consistent peak memory usage. We consider the following scenarios for peak memory determination:

\subsection{Depthwise-Dominated Scenario}
Assuming the depthwise convolution layer dominates memory usage in both current and next stages:

\begin{equation}
    M_{dw}(C_{in}) = M_{dw}(C_{out})
\end{equation}

Expanding and solving for $C_{out}$:

\begin{equation}
    C_{out} = C_{in} \cdot \frac{I^2 + 4K^2 + \frac{I^2}{4}}{2I^2 + 4K^2}
\end{equation}

\subsection{Depthwise to Expansion Transition}
When the peak transitions from depthwise to expansion layer:

\begin{equation}
    M_{dw}(C_{in}) = M_{exp}(C_{out})
\end{equation}

This leads to a quadratic equation in $C_{out}$:

\begin{equation}
    AC_{out}^2 + BC_{out} + D = 0
\end{equation}

where:
\begin{align*}
    A &= E \\
    B &= \frac{EI^2}{4} + \frac{I^2}{4} \\
    D &= -EC_{in}(I^2 + K^2 + \frac{I^2}{4})
\end{align*}

The solution is given by:

\begin{equation}
    C_{out} = \frac{-B + \sqrt{B^2 - 4AD}}{2A}
\end{equation}

\subsection{Expansion-Dominated Scenario}
When the expansion layer dominates in the current stage, there is only one possibility for the next stage: it must be dominated by the depthwise convolution layer.

\begin{equation}
    M_{exp}(C_{in}) = M_{exp}(C_{out})
\end{equation}

This also results in a quadratic equation:

\begin{equation}
    AC_{out}^2 + BC_{out} + D = 0
\end{equation}

where:
\begin{align*}
    A &= E \\
    B &= \frac{EI^2}{2} + \frac{I^2}{4} \\
    D &= -C_{in}(\frac{I^2}{4} + EC_{in} + EI^2)
\end{align*}

The solution follows the same form as in the previous scenario.

\subsection{Optimal Channel Size Selection}
To determine the optimal $C_{out}$, we select the appropriate value based on the current stage's dominant layer:

\begin{equation}
    C_{out}^* = \begin{cases}
        \min(C_{out,dw}, C_{out,dw-exp}) & \text{if depthwise dominates current stage} \\
        C_{out,exp-dw} & \text{if expansion dominates current stage}
    \end{cases}
\end{equation}

This approach ensures minimal memory usage while maintaining consistency across stages, taking into account the realistic transitions between dominant layers in consecutive stages.
